# Supplementary material for: GUI Testing Arena: A Unified Benchmark for Advancing Autonomous GUI Testing Agent
Source: arXiv:2412.18426 source file (2024-12-24)
Supplement: Supplementary file 1 [file X_suppl.tex]

\clearpage
\setcounter{page}{1}
\maketitlesupplementary

\tcbset{
  myboxstyle/.style={
    colback=gray!20,     
    colframe=black!70,    
    coltitle=white,       
    fonttitle=\bfseries,  
     fontupper=\itshape,
    boxrule=0.8mm,       
    arc=1mm,               
    boxsep=1mm,             
    left=1mm,              
    right=1mm,              
    top=1mm,               
    bottom=1mm,             
    toptitle=0mm,           
    bottomtitle=0mm,     
    enhanced,                  
  }
}

\section{Implementation Details}
Due to the page limit of the main paper, we provide more implementation details here. In §\ref{sec:local} and §\ref{sec:global+local},  we detail the implementation of Local Input and Global+Local Input, respectively. §\ref{sec:additional} describes the implementations common to both. Finally, based on the introductions in the first three subsections, we present the complete algorithm workflow of Zoom Eye in §\ref{sec:complete}.

\subsection{Local Input}\label{sec:local}
We select LLaVA-v1.5-7B~\cite{liu2024improved} and 13B as our MLLMs, with the vision encoder's input resolution as 336px and naive processing. We set the threshold of the stopping criterion at $\tau$ = 0.8 and define the weighted function as $\mathcal{W}$ = $ \frac{1-b}{D^2}\times d^2 + b $, where $D$ denotes the depth of the image tree, $d$ is the depth of the visited node during the search, and $b$ is a bias value, set here at 0.2. The prompt templates for calculating \textit{existing confidence}, \textit{latent confidence}, and \textit{answering confidence}~(please refer to §\ref{sec:confidence} and §\ref{sec:stop} for the discussion on these three confidence values) are set as:

\begin{tcolorbox}[myboxstyle, title=Prompt Templates of Local Input]
\begin{itemize}
\setlength{\itemsep}{6pt}\label{sec:global+local}
  \item $\text{p}_e(o)$: \textless local patch\textgreater\,Is there a $\{o\}$ in the image? Answer Yes or No.
  \item $\text{p}_l(o)$: \textless local patch\textgreater\,According to your common sense knowledge and the content of the image, is it possible to find a $\{o\}$ in the image? Answer Yes or No and tell the reason.
  \item $\text{p}_a(q)$: \textless local patch\textgreater\,Question: $\{q\}$ \textbackslash nCould you answer the question based on the the available visual information? Answer Yes or No.
\end{itemize}
\end{tcolorbox}

\noindent where the $o$ and $q$ are the input visual cue and question, which could be referred to §\ref{sec:algorithm} .

As mentioned in §\ref{sec:algorithm}, the final visual input uses the union of all searched patches. However, when multiple distant patches are combined, they may form a large image. For MLLMs using naive resize processing, information can still be lost during downsampling. Therefore, for the Local Input Zoom Eye with naive resize processing, when the area of  $b^*$  is relatively large (with the longer side exceeding 1000px), we skip the Union operation.  Instead, we paste the searched patches onto a blank image according to their relative positions in the original image, and then feed it to the MLLMs. An example is shown in Figure \ref{fig:patch paste}.

\begin{figure}[ht!]
    \centering
    \includegraphics[width=8.2cm]{author-kit-CVPR2025-v3-latex-/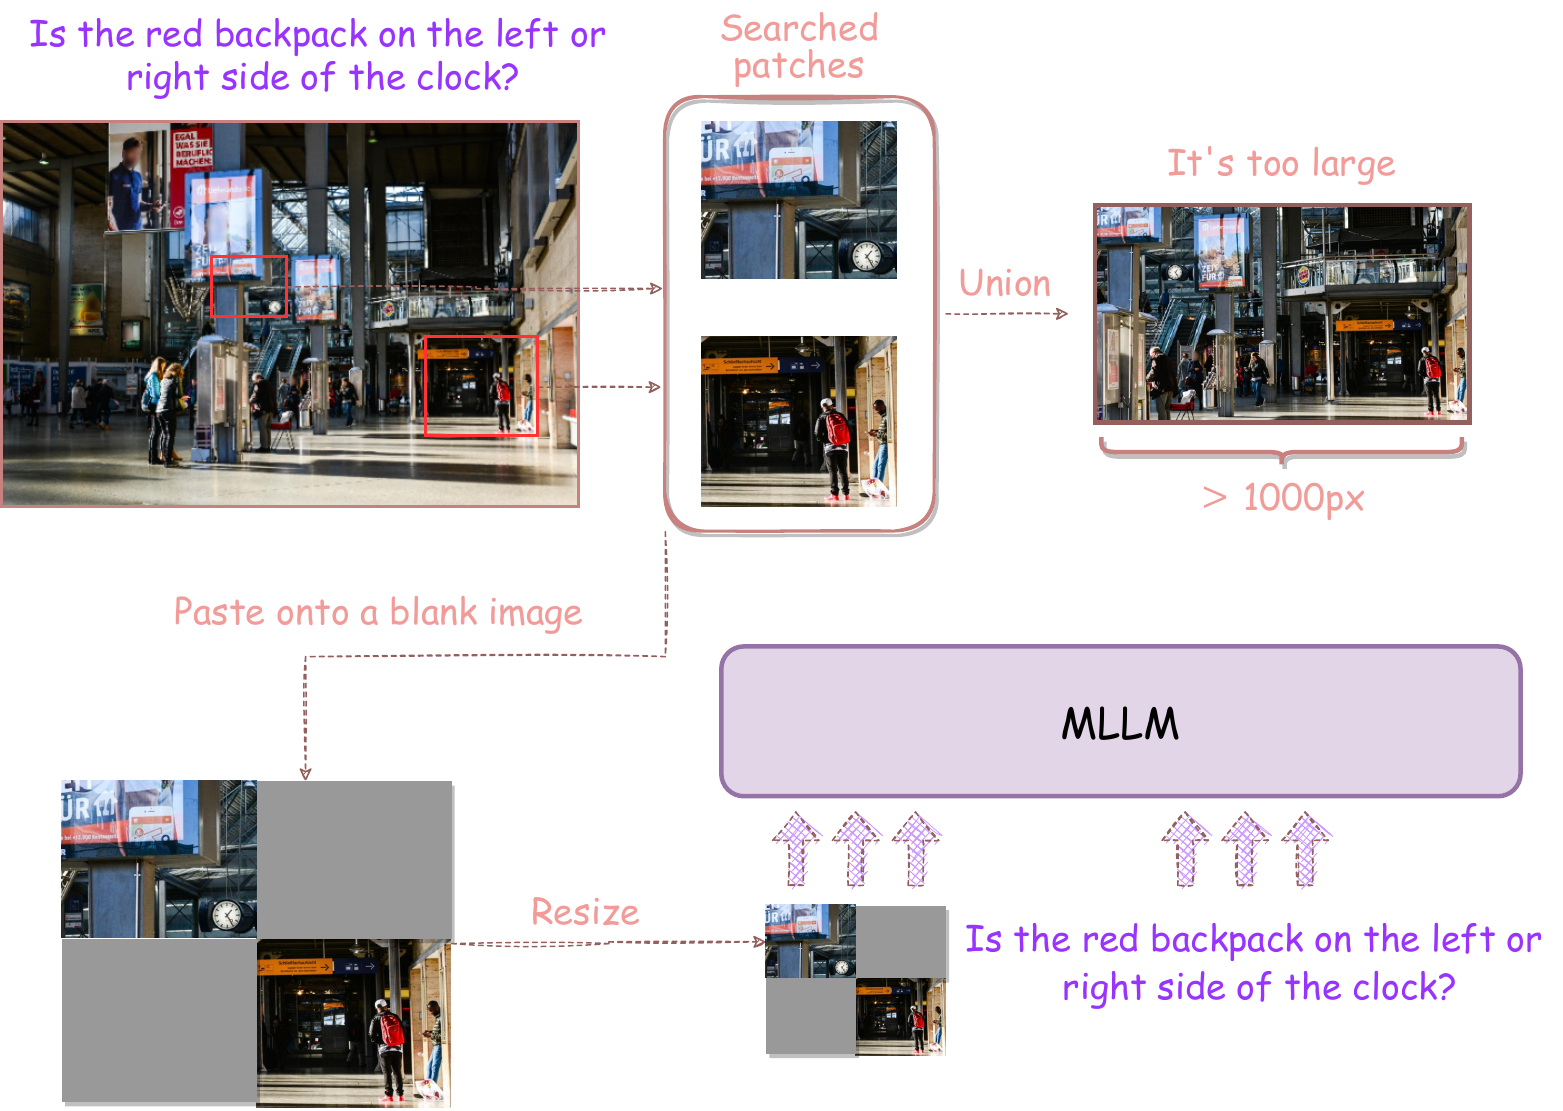}
    \caption{If the area of the union bounding box is too large, we paste the searched patches onto a blank image according to their relative positions in the original image, and then feed it to the MLLMs.\textbf{It is notable that this operation is only applied to Local Input, while for Local+Global, we consistently provide the MLLMs with the full union patch as input.}}
    \label{fig:patch paste}
\end{figure}

\subsection{Global\,+\,Local Input}\label{sec:global+local}
We select LLaVA-ov(oneVision)-0.5B~\cite{li2024llava} and 7B as our MLLMs, with the vision encoder's input resolution as 384px and AnyRes processing. We define the maximum AnyRes block as 12, set $\tau$ at 0.6 and define $\mathcal{W}$ as $ \frac{1-b}{D^2}\times d^2 + b $, where $D$ denotes the depth of the image tree, $d$ is the depth of the visited node during the search, and $b$ is a bias value, set here at 0.6. The prompt templates for calculating \textit{existing confidence}, \textit{latent confidence}, and \textit{answering confidence} are set as:

\begin{tcolorbox}[myboxstyle, title=Prompt Templates of Global\,+\,Local Input]
\begin{itemize}
\setlength{\itemsep}{6pt}
  \item $\text{p}_e(o)$: \textless global image\textgreater \textless local patch\textgreater\,Is there a $\{o\}$ in the zoomed-in view? Answer Yes or No.
  \item $\text{p}_l(o)$: \textless global image\textgreater \textless local patch\textgreater\,According to your common sense knowledge and the content of the zoomed-in view, along with its location in the image, is it possible to find a $\{o\}$ by further zooming in the current view? Answer Yes or No and tell the reason.
  \item $\text{p}_a(q)$: \textless global image\textgreater \textless local patch\textgreater\,Question: $\{q\}$ \textbackslash nCould you answer the question based on the the available visual information? Answer Yes or No.
\end{itemize}
\end{tcolorbox}

\subsection{Additional Settings}\label{sec:additional}
For both input implementation, we set the maximum search depth at 2 when searching for type\,2 cues to save costs. In §\ref{sec:algorithm}, we state that we search the whole tree to add all nodes with sufficient \textit{existing confidence} to $L$ if  type\,2 cue is generated. Thus, we introduce an additional threshold $\tau_2$ for this condition, which is set at 0.8 for both implementation. The decomposed question template $\text{p}_{dq}(o_i)$ is assigned as ``\texttt{What is the appearance of the $\{o_i\}$?}". For type\,1 search, a key aspect is determining the value of $\tau$. If it is set too low, an incorrect patch, which probably lead to erroneous guidance  for MLLMs, may be selected. Conversely, setting $\tau$ too high, surpassing the $c_a$ values of all nodes in the tree, would compel MLLMs to search the entire tree unnecessarily, thus wasting time. Therefore, we adopt a strategy where $\tau$ is progressively reduced as the number of search steps increases. Specifically, if the number of  search steps exceeds the step threshold $C$, we reduce the value of $\tau$ by 0.1. This reduction  occurs every $\delta$ steps, until the $c_a$ value of a node having been visited surpasses $\tau$ or $\tau$ falls below a predefined minimum limit $\tau_{min}$. For both implementation, we set $\delta$ at 2, $\tau_{min}$ at 0, and $C$ as $D\times3$. Finally, the in-context examples we utilized to generate visual cues are denote as $(q^{(1)},\textbf{o}^{(1)},\dots,q^{(m)},\textbf{o}^{(m)})$ and are presented at the end of this document.

\subsection{Complete Algorithm Workflow}\label{sec:complete}

With the above notations and definitions in place, we provide the complete algorithm workflow in Algorithm \ref{algorithm:complete}, where the Zoom Eye search method is shown in Algorithm \ref{algorithm:zoom eye}.

\begin{algorithm}
\caption{Complete Algorithm Workflow of Zoom Eye}
\small
\begin{algorithmic}[1]
\Require Multimodal LLM $\Phi_{\theta}$, input question-image pair (\textbf{I}, $q$), decomposed question template $\text{p}_{dq}$, in-context examples $(q^{(1)},\textbf{o}^{(1)},\dots,q^{(m)},\textbf{o}^{(m)},q)$
\State $\{o_1,\dots,o_k\} \gets \Phi_{\theta}.\text{generate}(q^{(1)},\textbf{o}^{(1)},\dots,q^{(m)},\textbf{o}^{(m)},q)$
\State  Initialize $L$ as the empty list
\State  Build \textbf{I} as a tree $T$
\For{$i=1,\dots,k$}
    \If{$k==1$}
        \State $q_s \gets q$
    \Else
        \State $q_s \gets \text{p}_{dq}(o_i)$
    \EndIf
    \State $L$.extend(\Call{Zoom Eye}{$T, o_i, q_s$})
\EndFor
\State $\textbf{b}^* \gets \text{Union bounding-boxes of all nodes in } L$
\State $n^* \gets \{\textbf{I}, \textbf{b}^*\}$
\State Final response $\gets \Phi_{\theta}.\text{generate}(\mathcal{V}(n^*),q)$
\end{algorithmic}\label{algorithm:complete}
\end{algorithm}

\begin{algorithm}
\caption{Zoom Eye Search}
\small
\begin{algorithmic}[1] % The number [1] here means every line will be numbered
\Require{Threshold of type 1 cue and type 2 cue ($\tau, \tau_2$), minimum limit $\tau_{min}$, interval $\delta $}
\Function{Zoom Eye}{\;$T,o_i,q_s$}
    \State Initialize $Q$ as the empty queue \{\}
    \State $Q$.\texttt{append($T$.root)}
    \State Initialize $L_i$ as the empty list
    \State search all $\gets$ $o_i$.\texttt{startswith}(``all")
    \If{not search all}
        \State \Call{Zoom Eye Type 1}{\;$T,Q,L_i,q_s,\tau$}
    \Else
        \State \Call{Zoom Eye Type 2}{\;$Q,L_i,\tau_2$}
    \EndIf
    \State \Return{$L_i$}
\EndFunction
\State
\Function{Zoom Eye Type 1}{\;$T,Q,L_i,q_s,\tau$}
    \State import $\mathcal{R}$ and $\mathcal{S}$ from Algorithm \ref{algorithm:rank}
    \State count $\gets$ 0
    \State $C \gets T.depth \times 3$
    \State Initialize $n_m$ as $T$.root to record the node with the best $c_a$
    \While{$Q$ is not empty}
        \State $n_t \gets Q.\texttt{pop()}$
        \State $N$.\texttt{append}($n_t$)
        \State count $\gets$ count + 1
        \If{count $\geq$ C}
            \State $\tau \gets \tau - 0.1$
            \State $C \gets C+\delta$
            \If{$\tau < \tau_{min}$}
                \State \textbf{break}
            \EndIf
        \EndIf
        \If{$\mathcal{S}(n_t,q_s,\tau)==\text{True}$}
            \State $L_i$.\texttt{append}($n_t$)
            \State \textbf{break}
        \ElsIf{$\mathcal{S}(n_m,q_s,\tau)==\text{True}$}
            \State $L_i$.\texttt{append}($n_m$)
            \State \textbf{break}
        \EndIf
        \If{$n_t.c_a \geq n_m.c_a$}
            \State $n_m \gets n_t$
        \EndIf
        \State $s \gets n_t.\texttt{children.size}$
        \For{$j=1,\dots,s$}
            \State $Q$.\texttt{append($n_t$.children[j])}
        \EndFor
        \State $Q$.\texttt{sort($\mathcal{R}(o_i)$)}
    \EndWhile
\EndFunction
\State
\Function{Zoom Eye Type 2}{\;$Q,L_i,\tau_2$}
    \While{$Q$ is not empty}
        \If{$n_t.\texttt{depth} \geq 2$}
            \State \textbf{break}
        \EndIf
        \State $c_e$ $\gets$ calculate the existing confidence of $n_t$
        \If{$c_e \geq \tau_2$}
            \State $L_i$.\texttt{append}($n_t$)
        \EndIf
        \State $s \gets n_t.\texttt{children.size}$
        \For{$j=1,\dots,s$}
            \State $Q$.\texttt{append($n_t$.children[j])}
        \EndFor
    \EndWhile
\EndFunction
\end{algorithmic}\label{algorithm:zoom eye}
\end{algorithm}

\section{Results on MME-RealWorld Benchmark}

We provide the complete results of Zoom Eye on MME-RealWorld Benchmark~\cite{zhang2024mme}, as show in Table \ref{table:mme all}. This benchmark includes 5 data categories: Monitoring\;(MO), Autonomous Driving\;(AD), OCR, emote Sensing\;(RS), and Diagram and Table\;(TD). Since Zoom Eye is not applicable to the TD task,  we do not conduct tests on it. It could be observed that Zoom Eye improves the performance of LLaVA-ov-7B across most sub-tasks, with particularly significant improvements in certain tasks. For instance, it achieves a 20.22\% improvement in the Person$_\text{{color}}$ task, a 29.11\% improvement in the Motion$_\text{{vehicle}}$ task, and a 12.93\% improvement in the Visual$_\text{{trafficsignal}}$  task, demonstrating the effectiveness of Zoom Eye. However, performance declines were observed in some sub-tasks when using Zoom Eye. We have analyzed these cases in the main paper, revealing certain limitations of the employed MLLM. Addressing these issues will be a focus of our future work.

\begin{table}[h!]
\footnotesize
  \begin{center}
  \resizebox{\hsize}{!}{
  \setlength\tabcolsep{2pt}
    \begin{tabular}{l c c c c c r} 
    \toprule
      \textbf{Task} &  & & & LLaVA$_{\text{ov}}$-7B & +ZoomEye & \;$\Delta\uparrow$ \\
    \midrule
      \multirow{10}{*}{\textbf{MO}} & \vline & Calculate & \vline & 36.33 & 38.67 & \textcolor{darkgreen}{+2.34} \\
                  & \vline & Intention & \vline  & 27.55 & 38.78 & \textcolor{darkgreen}{+11.23}\\
                  & \vline & Property & \vline  & 55.0 & 60.0 & \textcolor{darkgreen}{+5.0}\\
                  & \vline & Vehicle$_{\text{counting}}$ & \vline  & 59.89 & 61.14 &\textcolor{darkgreen}{+1.25} \\
                  & \vline & Person$_{\text{counting}}$ & \vline  & 61.35 & 61.87 & \textcolor{darkgreen}{+0.52}\\
                  & \vline & Vehicle$_{\text{location}}$ & \vline  & 33.82 & 33.82 &  -\\
                  & \vline & Vehicle$_{\text{orientation}}$ & \vline  & 19.35 & 18.71 & \textcolor{red}{-0.64}\\
                  & \vline & Vehicle$_{\text{color}}$ & \vline  & 43.65 & 49.24 & \textcolor{darkgreen}{+5.59}\\
                  & \vline & Person$_{\text{color}}$ & \vline  & 24.72 & 44.94 & \textcolor{darkgreen}{+20.22}\\
                  & \vline & Person$_{\text{orientation}}$ & \vline  & 10.53 & 10.53 & - \\
    \midrule
      \multirow{15}{*}{\textbf{AD}} & \vline & Intention$_{\text{ego}}$ & \vline  & 28.62 & 28.95 & \textcolor{darkgreen}{+0.33} \\
                  & \vline & Intention$_{\text{pedestrian}}$ & \vline  & 52.43 & 53.40 & \textcolor{darkgreen}{+0.97} \\
                  & \vline & Intention$_{\text{vehicle}}$ & \vline  & 30.92 & 33.33 & \textcolor{darkgreen}{+2.41} \\
                  & \vline & Interaction$_{\text{other2other}}$ & \vline  & 12.94 & 13.43 & \textcolor{darkgreen}{+0.49} \\
                  & \vline & Attention$_{\text{trafficsignal}}$ & \vline  & 71.89 & 68.66 & \textcolor{red}{-3.23} \\
                  & \vline & Interaction$_{\text{ego2pedestrain}}$ & \vline  & 27.36 & 28.30 &\textcolor{darkgreen}{+0.94} \\
                  & \vline & Interaction$_{\text{ego2trafficsignal}}$ & \vline  & 22.86 & 25.71 & \textcolor{darkgreen}{+2.85} \\
                  & \vline & Interaction$_{\text{ego2vehicle}}$ & \vline  & 20.79 & 19.80 & \textcolor{red}{-0.99} \\
                  & \vline & Objects$_{\text{identify}}$ & \vline  & 64.40 & 64.85 & \textcolor{darkgreen}{+0.45} \\
                  & \vline & Motion$_{\text{vehicle}}$ & \vline  & 23.42 & 52.53 & \textcolor{darkgreen}{+29.11} \\
                  & \vline & Motion$_{\text{multivehicles}}$ & \vline  & 34.26 & 34.75 & \textcolor{darkgreen}{+0.49} \\
                  & \vline & Visual$_{\text{trafficsignal}}$ & \vline  & 60.20 & 73.13 & \textcolor{darkgreen}{+12.93} \\
                  & \vline & Motion$_{\text{pedestrain}}$ & \vline  & 34.15 & 40.85 & \textcolor{darkgreen}{+6.70} \\
                  & \vline & Object$_{\text{count}}$ & \vline  & 37.92 & 39.86 & \textcolor{darkgreen}{+1.94} \\
                  & \vline & Motion$_{\text{multipedestrians}}$ & \vline  & 31.24 & 31.64 & \textcolor{darkgreen}{+0.40} \\
    \midrule
     \multirow{7}{*}{\textbf{OCR}}             & \vline & Scene understanding & \vline  & 64.80 & 64.80 & - \\
                  & \vline & Character identification & \vline  & 57.60 & 56.40 & \textcolor{red}{-1.20}\\
                  & \vline & Adver \& product & \vline  & 76.64 & 78.37 & \textcolor{darkgreen}{+1.73} \\
                  & \vline & Book map poster & \vline  & 77.17 & 75.24 & \textcolor{red}{-1.93} \\
                  & \vline & License & \vline  & 80.16 & 82.39 & \textcolor{darkgreen}{+2.23} \\
                  & \vline &  Phone \& address & \vline  & 77.82 & 81.28 & \textcolor{darkgreen}{+3.46} \\
                  & \vline & Text recog & \vline  & 74.87 & 77.13 & \textcolor{darkgreen}{+2.26} \\
    \midrule
      \multirow{3}{*}{\textbf{RS}}          & \vline & Color & \vline  & 59.60 & 60.56 & \textcolor{darkgreen}{+0.96} \\
                & \vline & Count & \vline  & 32.95 & 35.56 & \textcolor{darkgreen}{+2.61}\\
                & \vline &  Position & \vline  & 61.40 & 48.45 & \textcolor{red}{-12.95} \\
    \bottomrule
    \end{tabular}
    }
  \end{center}
  \caption{Performance comparison between Zoom Eye and the baseline model on MME-RealWorld benchmark. MO (Monitoring), AD (Autonomous Driving), OCR and RS (Remote Sensing) are data categories within this benchmark.}
  \label{table:mme all}
\end{table}

\begin{tcolorbox}[myboxstyle, title=In-Context Examples of $V^*$ Bench]
\begin{itemize}[label={}]
\setlength{\itemsep}{6pt}
  \item \textbf{User:} Question: What is the color of the boy's bag? If you want to answer the question, which objects' information do you need?
  \item \textbf{Assistant:} To answer the question, I need know the location of the boy with a bag so that I can determine the color of the bag. So I need the information about the following objects: boy with a bag.
  \item \textbf{User:} Is the yellow car on the left or right side of the white car?
  \item \textbf{Assistant:} To answer the question, I need know the location of the yellow car and the white car so that I can determine the positional relationship between the two of them. So I need the information about the following objects: white car and yellow car.
  \item \textbf{User:} Tell me the number on the black board.
  \item \textbf{Assistant:} To answer the question, I need know the location of the black board so that I can determine the number on it. So I need the information about the following objects: black board
  \item \textbf{User:} Is the girl with pink hair on the left or right side of the man with backpack?
  \item \textbf{Assistant:} To answer the question, I need know the location of the girl with pink hair and the man with backpack so that I can determine the positional relationship between the two of them. So I need the information about the following objects: girl with pink hair and man with backpack.
  \item \textbf{User:} What kind of animal is on the red sign?
  \item \textbf{Assistant:} To answer the question, I need know the location of the red sign so that I can determine the kind of animal on it. So I need the information about the following objects: red sign.
  \item \textbf{User:} From the information on that advertising board, what is the type of this shop?
  \item \textbf{Assistant:} To answer the question, I need know the location of the advertising board so that I can determine the type of the shop. So I need the information about the following objects: advertising board.
\end{itemize}
\end{tcolorbox}

\begin{tcolorbox}[myboxstyle, title=In-Context Examples of HR-Bench]
\begin{itemize}[label={}]
\setlength{\itemsep}{6pt}
  \item \textbf{User:} Question: What is the color of the boy's bag? If you want to answer the question, which objects' information do you need?
  \item \textbf{Assistant:} To answer the question, I need know the location of the boy with a bag so that I can determine the color of the bag. So I need the information about the following objects: boy with a bag.
  \item \textbf{User:} Is the yellow car on the left or right side of the white car?
  \item \textbf{Assistant:} To answer the question, I need know the location of the yellow car and the white car so that I can determine the positional relationship between the two of them. So I need the information about the following objects: white car and yellow car.
  \item \textbf{User:} Tell me the number on the black board above the dog.
  \item \textbf{Assistant:} To answer the question, I need know the location of the black board above the dog so that I can determine the number on it. So I need the information about the following objects: black board above the dog.
  \item \textbf{User:} Is the girl with pink hair on the left or right side of the man with backpack?
  \item \textbf{Assistant:} To answer the question, I need know the location of the girl with pink hair and the man with backpack so that I can determine the positional relationship between the two of them. So I need the information about the following objects: girl with pink hair and man with backpack.
  \item \textbf{User:} What kind of animal is on the red sign?
  \item \textbf{Assistant:} To answer the question, I need know the location of the red sign so that I can determine the kind of animal on it. So I need the information about the following objects: red sign.
  \item \textbf{User:} How many cars in the image?
  \item \textbf{Assistant:} To answer the question, I need know the location of all cars so that I can determine the number of cars. So I need the information about the following objects: all cars.
  
\end{itemize}
\end{tcolorbox}
